# Supplementary material for: Coordinated Multi-Robot Shared Autonomy Based on Scheduling and Demonstrations
Source: arXiv:2303.15972 source file (2023-10-25)
Supplement: Supplementary file 1 [file 06_appendix.tex]

\section{Evaluation Parameters}
\label{app:parameters}
In this appendix, we provide the values of parameters used for all parts of the method and evaluation. For simplicity, when choosing weights to align demonstrations in the time warping, we used only the Cartesian variables with equal weights (i.e., $x$, $y$, and $z$). The augmented robot state consisted of 11 state variables including the position, orientation (represented as a quaternion), force, valve state, and time warp gradient variable. While the four entries of the quaternion are coupled, our changes in orientation were sufficiently small such that an interpolation and re-normalization procedure was sufficient. The weights for the principal component analysis were based on setting the expected range, $r$, of each state variable. The weight was then calculated as the squared inverse (i.e., $w = \frac{1}{r^2}$) to match the squared units of Equation \ref{eq:variancefromdemos}.

\begin{center}
\begin{table}[H]
\centering
\caption{Parameters used in Method}
\label{table:parameters}
\begin{tabular}{cccc} \toprule
    \multicolumn{4}{c}{\textbf{Corrections from Variance}}\\ \midrule
    \textit{Parameter} & \textit{Value} & \textit{Parameter} & \textit{Value}\\ \midrule
    $r_x$ & $2$ & $r_y$ & $2$  \\
    $r_z$ & $2$ & $r_{q_x}$ & $1$  \\
    $r_{q_y}$ & $1$ & $r_{q_z}$ & $1$  \\
    $r_{q_w}$ & $1$ & $r_{f_x}$ & $30$  \\
    $r_{f_y}$ & $30$ & $r_{f_z}$ & $30$  \\
    $r_{valve}$ & $1$ & $r_{\dot{\psi}_\mathcal{D}}$ & $1$  \\ \midrule
    \multicolumn{4}{c}{\textbf{Bayesian Inference}}\\ \midrule
    \textit{Parameter} & \textit{Value} & \textit{Parameter} & \textit{Value}\\ \midrule
    $\gamma_p$  & $20$ & $\sigma^{2}_{\textrm{MAX}}$ & $0.1$  \\ 
    $\mu_c$ & $0.5$ & $\gamma_c$ & $0.9$   \\
    $\epsilon$ & $1e-6$ \\ \bottomrule
\end{tabular}
\end{table}
\end{center}

In Table \ref{table:parameters}, we report both the ranges used for each state variable in principal component analysis of the variability (i.e., corrections) and the parameters used for the Bayesian Inference. The parameters chosen for the Bayesian Inference directly impact the required number of executions to achieve high confidence. Other values may be more appropriate depending on the application and criticality. The sample rate, $\Delta t_s$, was 0.2 seconds for all demonstrations and executions. All of the parameters were fixed prior to collecting the final demonstrations used in the evaluation.
